# Supplementary material for: LQER: Low-Rank Quantization Error Reconstruction for LLMs
Source: arXiv:2402.02446 source file (2024-05-30)
Supplement: Supplementary file 1 [file appendix-sgl-val-dist.tex]

\begin{figure*}
    \vskip 0.2in
    \begin{center}
        \begin{subfigure}{0.24\linewidth}
            \centering
            \includegraphics[width=\linewidth]{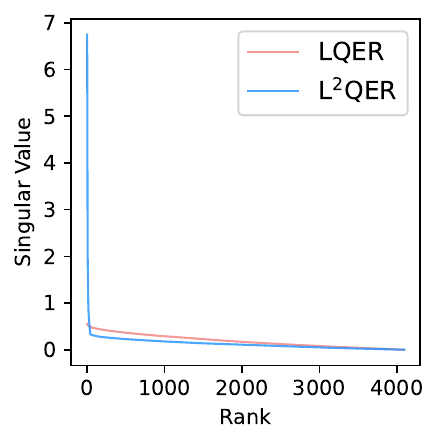}
            \caption{The 4th K layer}
            \label{fig:appendix:sgl_vals_dist:layer_4_k}
        \end{subfigure}
        \begin{subfigure}{0.24\linewidth}
            \centering
            \includegraphics[width=\linewidth]{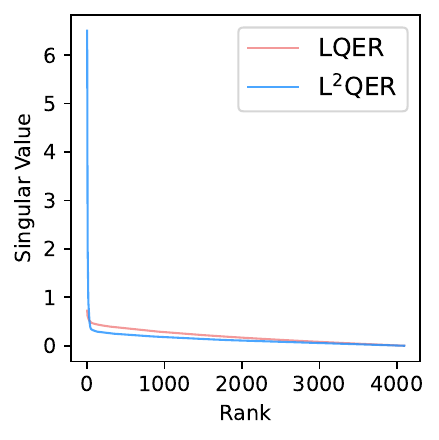}
            \caption{The 4th Q layer}
            \label{fig:appendix:sgl_vals_dist:layer_4_q}
        \end{subfigure}
        \begin{subfigure}{0.24\linewidth}
            \centering
            \includegraphics[width=\linewidth]{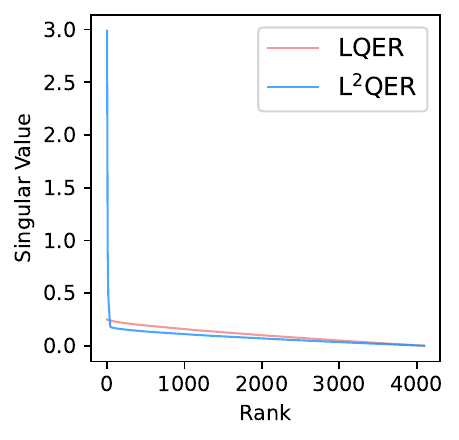}
            \caption{The 4th V layer}
            \label{fig:appendix:sgl_vals_dist:layer_4_v}
        \end{subfigure}
        \begin{subfigure}{0.24\linewidth}
            \centering
            \includegraphics[width=\linewidth]{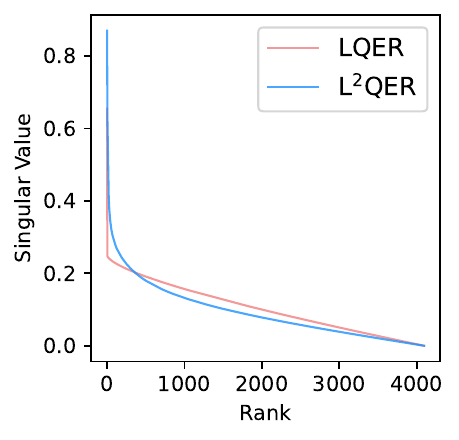}
            \caption{The 4th O layer}
            \label{fig:appendix:sgl_vals_dist:layer_4_o}
        \end{subfigure}

        \begin{subfigure}{0.24\linewidth}
            \centering
            \includegraphics[width=\linewidth]{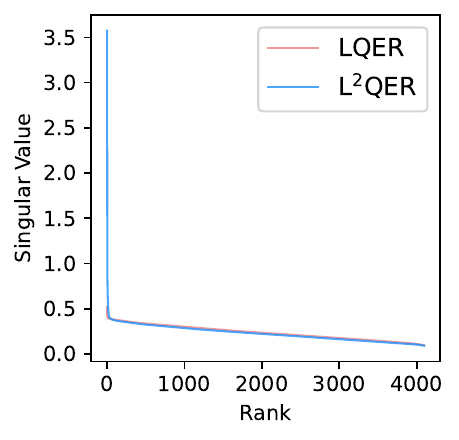}
            \caption{The 4th Up layer}
            \label{fig:appendix:sgl_vals_dist:layer_4_up}
        \end{subfigure}
        \begin{subfigure}{0.24\linewidth}
            \centering
            \includegraphics[width=\linewidth]{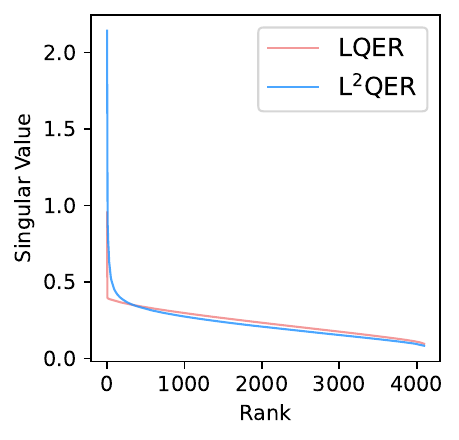}
            \caption{The 4th Down layer}
            \label{fig:appendix:sgl_vals_dist:layer_4_down}
        \end{subfigure}
        \begin{subfigure}{0.24\linewidth}
            \centering
            \includegraphics[width=\linewidth]{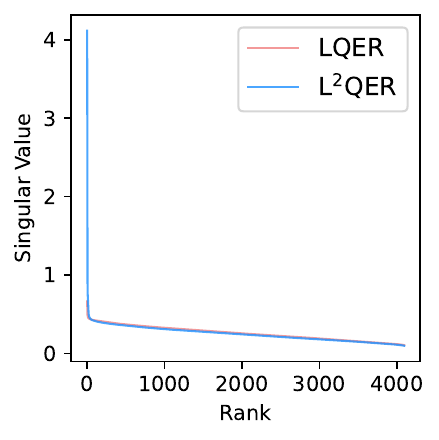}
            \caption{The 4th Gate layer}
            \label{fig:appendix:sgl_vals_dist:layer_4_gate}
        \end{subfigure}
        \begin{subfigure}{0.24\linewidth}
            \centering
            \includegraphics[width=\linewidth]{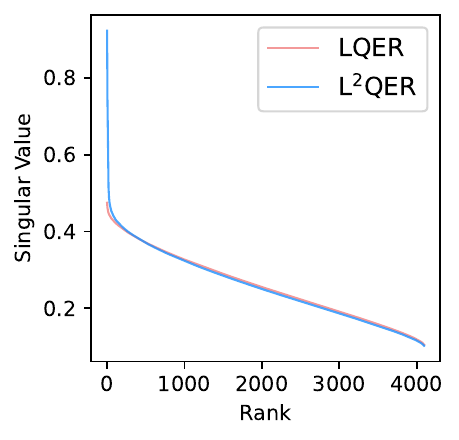}
            \caption{The 19th Gate layer}
            \label{fig:appendix:sgl_vals_dist:layer_19_gate}
        \end{subfigure}

        \vskip -0.1in
        \caption{The singular value distributions of \LRQn{} and \LRQa{}. We find that the shaping effect of \LRQa{} are obvious on most layers in LLaMA. Most O projection layers and several layers at the beginning or the end of the model tend to have an $E_q$ distribution decaying slowly (See~\Cref{fig:appendix:sgl_vals_dist:layer_4_o} and \Cref{fig:appendix:sgl_vals_dist:layer_19_gate}).
        }
        \label{fig:appendix:sgl_vals_dist}
    \end{center}
    \vskip -0.2in
\end{figure*}
