# Supplementary material for: LQER: Low-Rank Quantization Error Reconstruction for LLMs
Source: arXiv:2402.02446 source file (2024-05-30)
Supplement: Supplementary file 2 [file appendix-Eq-distribution-vs-bitwidth.tex]

\begin{figure*}
    \vskip 0.2in
    \begin{center}
        \includegraphics[width=\textwidth]{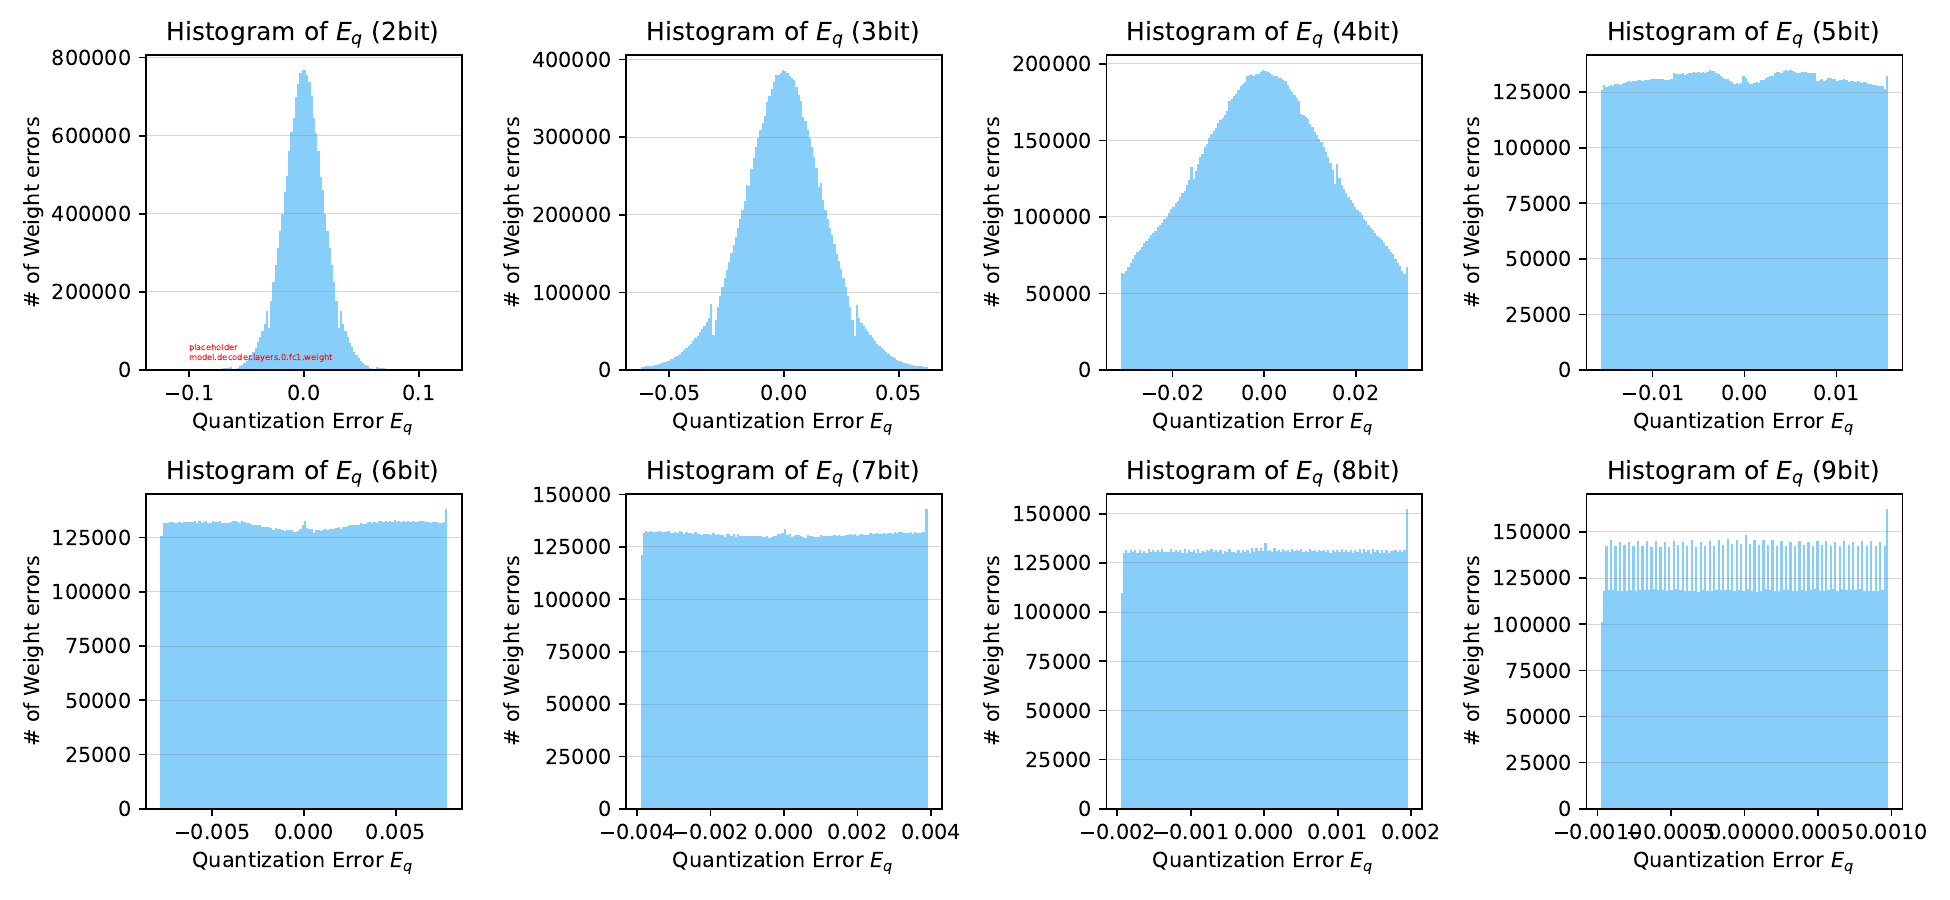}
        \caption{Distribution of quantization errors $E_q$ for different bitwidths. We observe that low-precision like 2-bit or 3-bit fixed-point quantization creates a random matrix $E_q$ close to Gaussian distribution, while relatively high precision fixed-point quantization creates a $E_q$ close to uniform distribution.}
        \label{fig:s4:q-error-histogram-vs-bitwidth}
    \end{center}
    \vskip -0.2in
\end{figure*}
